# Supplementary material for: sharpDARTS: Faster and More Accurate Differentiable Architecture Search
Source: arXiv:1903.09900 source file (2019-03-23)
Supplement: Supplementary file 1 [file arxiv_appendices.tex]

\appendix
